# Supplementary material for: Probabilistic ODE Solvers with Runge-Kutta Means
Source: arXiv:1406.2582 source file (2014-10-24)
Supplement: Supplementary file 1 [file appendix.tex]

\section{Appendix}
\subsection{General kernel derivatives of stationary kernels}

\emph{Stationary kernels} can be written as a function of the distance, i.e.,
$k(t,t') = \tilde{k}(|t-t'|)$. In many cases, it is helpful to define the
distance in terms of the squared distance and in units of the step length $h$.
\begin{align}
r(t,t') &= \frac{(t-t')^2}{h^2}\\
k(t,t') &= (\tilde{k} \circ r)(t,t')
\end{align}

In the following, there is a list of necessary kernel derivatives in order to
compute partial kernel derivatives needed in Sec.~\ref{sec:2nd-order-methods}.
We will write $k(r)$ for $\tilde{k}(r(t,t'))$ for easier parsing.

\begin{align}
\kd  &= \dkdr \frac{\de r}{\de t'}\\
\label{eq:kd-stat}
     &= \dkdr \left(-2\frac{(t-t')}{h^2}\right)\\
\dkd &= \frac{\de \kd}{\de t}\\
     &= \left(\dtkdrt \frac{\de r}{\de t} \frac{\de r}{\de t'}\right)
      + \left(\dkdr \frac{\de^2 r}{\de t \de t'}\right)\\
\label{eq:dkd-stat}
     &= -4 \frac{(t-t')^2}{h^4} \dtkdrt - \frac{2}{h^2} \dkdr
\end{align}

With Eqs.~\eqref{eq:kd-stat} and \eqref{eq:dkd-stat}, this gives rise to the
following substitutions:
\begin{align}
k(t_n + h\alpha, t_n + h\alpha) &= k(0)\\
\kd(t_n + h\alpha, t_n) &= -2\frac{\alpha}{h} \evalat{\dkdr}{\alpha^2}\\
\kd(t_n + h, t_n) &= -\frac{2}{h} \evalat{\dkdr}{1}\\
\kd(t_n + h, t_n + h\alpha) &= -2 \frac{(1-\alpha)}{h} \evalat{\dkdr}{(1-\alpha)^2}\\
\dkd(t_n + h\alpha, t_n + h\alpha) &= - \frac{2}{h^2} \evalat{\dkdr}{0}\\
\dkd(t_n, t_n) &= - \frac{2}{h^2} \evalat{\dkdr}{0}\\
\dkd(t_n + h\alpha, t_n) &= -4 \frac{\alpha^2}{h^2} \evalat{\dtkdrt}{\alpha^2} 
                             - \frac{2}{h^2}\evalat{\dkdr}{\alpha^2}
\end{align}

Furthermore, we observe that there are two special cases, $\alpha = \frac{1}{2}$
and $\alpha = 1$, which need to be treated seperately.

\subsection{The Integrated Wiener Process}
It was assumed that the Integrated Wiener Process (IW) will lead to a connection with
Runge-Kutta methods. This section details the derivation of
higher-order IW kernels, derivatives and other needed relationships.

The \emph{Wiener Process kernel} is given by:
\begin{align}
k_{WP}(t,t') &= c (\min(t,t') - b)
\end{align}
In order to arrive at higher-order IW kernels, one must integrate
$k_{WP}$ with respect to both $t$ and $t'$ which gives:
\begin{align}
k^1_{WP}(t,t') &= \int_b^t du \int_b^{t'} dv (c \min(u,v) - b)\\
&= c \int_b^t du \int_b^{t'} dv \min(u,v) - c b (t-b) (t'-b)\\
&\stackrel{t>t'}{=} c \left(\int_{t'}^t du \int_b^{t'} dv\; v 
                      + 2 \int_b^{t'} du \int_b^{u} dv\; v\right) 
                 - c b (t-b) (t'-b)\\
&= c \left( \int_{t'}^t du\; \frac{1}{2}(t'^2 - b^2) 
          + 2 \int_b^{t'} du\; \frac{1}{2} (u^2 - b^2) \right) - c b
          (t-b) (t'-b)\\
&= c \left( \frac{1}{2}(t-t')(t'^2 - b^2) - b^2 (t'-b) +
          \frac{1}{3}(t'^3 - b^3) \right) - c b (t-b)(t'-b)\\
% maybe include more intermediate steps here
&= c \left[ \abs{t - t'} \frac{\min\nolimits^2(t,t')}{2} +
            \frac{\min\nolimits^3(t,t')}{3} + \frac{1}{2} b^2(t+t') -
            \frac{1}{3}b^3 - btt'\right] 
\end{align}

Its derivatives are given by:
\begin{align}
\kd^1(t,t') &= 
  c \left[ 
    \begin{cases}
      t < t': & \frac{t^2}{2} + \frac{b^2}{2} - bt\\
      t > t': & tt' - \frac{t'^2}{2} + \frac{b^2}{2} - bt
    \end{cases}  
    \right]
\end{align}
and
\begin{align}
\dkd^1(t,t') &= c (\min(t,t') - b)
\end{align}
which is exactly what we expected it to be.

Iterating this process leads to the \emph{Twice Integrated Wiener
  Process}. For simplicity, we'll assume $b=0$  which leads to:
\begin{align}
k^2_{WP}(t,t') &= c \left[ \int_0^t du \int_0^{t'} dv\; \abs{u-v}
  \frac{\min\nolimits^2(u,v)}{2} +
  \frac{\min\nolimits^3(u,v)}{3}\right]\\
  &\stackrel{t>t'}{=} c \left[ 
     \left( \int_{t'}^t du \int_0^{t'} dv\; (u-v)
     \frac{v^2}{2} + \frac{v^3}{3} \right) + 
     \left( \int_0^{t'} du \int_0^u dv\; (u-v) \frac{v^2}{2} +
     \frac{v^3}{3} \right)  +
     \left( \int_0^v du \int_0^{t'} dv\; (v-u) \frac{u^2}{2} +
     \frac{u^3}{3} \right) \right]
\end{align}

\section{Basic derivatives}
The following derivatives are needed in computing some of the
derivatives of the \emph{Integrated Wiener Process}:
\begin{align}
\frac{\de}{\de t'} \abs{t - t'} &= \frac{\de}{\de t'} \sqrt{(t-t')^2}\\
&= \frac{1}{2 \sqrt{(t-t')^2}} 2 (t-t')(-1)\\
&= -\frac{(t-t')}{\sqrt{(t-t')^2}}\\
&= -\frac{(t-t')}{\abs{t-t'}}
\end{align}
Furthermore, we have:
\begin{align}
\frac{\de}{\de t'} \min(t, t') &= \frac{\de}{\de t'} \frac{1}{2} (t + t' - \abs{t - t'})\\
\label{eq:min-derivative}
&= \frac{1}{2}\left(1 + \frac{(t-t')}{\abs{t-t'}}\right)\\
&= \ind{[t > t']}
\end{align}

\section{Higher order integrated Wiener Process as solutions to
  Stochastic Differential Equations}

Consider a $d$-dimensional stochastic process
$\vec{X}(t) = (X_1(t), \dots, X_d(t))$ which satisfies the following
stochastic differential equations:
\begin{align}
d\vec{X}(t) &= \mat{F}\vec{X}(t) + \vec{L}d\vec{W}(t)
\end{align}
where $\vec{W}(t)$ denotes Brownian motion and $\mat{F}$ and $\vec{L}$
are mixing weights given in matrix and vector form. If $\mat{F}$ and
$\vec{L}$ are of the form
\begin{align}
\mat{F} &= \begin{bmatrix} 0 & 1 & 0 & \hdots & 0\\
                           0 & 0 & 1 & \hdots & 0\\
                           \vdots & \vdots & \ddots & \ddots & 0\\
                           0 & \hdots & \hdots & 0 & 1\\
                           0 & \hdots & \hdots & \hdots & 0
           \end{bmatrix}
&
\vec{L} &= \begin{bmatrix} 0\\ 0\\ \vdots\\ 0\\ 1 \end{bmatrix}
\end{align}
then it is clear that $X_d(t)$ is distributed according to a Brownian
motion but is also the $d^{\text{th}}$ derivative of $X_1(t)$ and,
therefore, $X_1(t)$ is a $d$-times integrated Brownian motion. This is
can be used to compute the covariance function of the $d$-times
integrated Wiener Process in closed form easily.
